# Supplementary material for: Revisiting the Implied Remaining Variance framework of Carr and Sun (2014): Locally consistent dynamics and sandwiched martingales
Source: arXiv:2105.06390 source file (2021-05-13)
Supplement: Supplementary file 1 [file Market_with_2_call.tex]

\subsection{Market with two call options}
Assume that on the market described in Example~\ref{ex:single} there exist two call options with strike prices $L$ and $K$, with $0 < L < K$.  Such a market is arbitrage-free on $[0,\tau] \cup \{T\}$ if $C^{\tau}(L), C^{\tau}(K)$ are two sandwiched martingales such that:
\begin{itemize}
	\item $C^{\tau}_t(L) \in \Big(\big(S_{t \wedge \tau} - L\big)_+, S_{t \wedge \tau}\Big)$;
	\item $C^{\tau}_t(K) \in \Big(\big(S_{t \wedge \tau} - K\big)_+, S_{t \wedge \tau}\Big)$;
	\item $ -1 < \frac{S_{t \wedge \tau} - C^{\tau}_t(L)}{0-L} < \frac{C^{\tau}_t(L) - C^{\tau}_t(K)}{L - K} < 0$, which entails $C^{\tau}_t(K) < C^{\tau}_t(L)$.
\end{itemize}

\subsubsection*{Assume $S_0 < L < K$ and define $\tau := \inf \big\{ t \in (0,T): S_t = L \big\}$. }
By continuity of $S$, it is
\[
\begin{cases}
	< L & \text{if $t < \tau$} \\
	= L & \text{if $t = \tau$}
\end{cases}.
\]
The convexity constraint requires
\[
-1 < \frac{S_{t \wedge \tau} - C^{\tau}_t(L)}{0-L} < 0 \quad \Longleftrightarrow \quad 0 < S_{t \wedge \tau} - C^{\tau}_t(L) < L \quad \Longleftrightarrow \quad S_{t \wedge \tau} - L < 0 < C^{\tau}_t(L) < S_{t \wedge \tau}
\]
so that if we set, as in the single call case,
\begin{equation}
C^{\tau}_t(L) = (S_{t \wedge \tau}-L)_+ + N_{t \wedge \tau}(L) \cdot \big[S_{t \wedge \tau} - (S_{t \wedge \tau}-L)_+\big] = N_{t \wedge \tau}(L) \cdot S_{t \wedge \tau}
\end{equation}
where $N_t(L)$ is an independent positive martingale independent of $W$ and unit-bounded, the convexity constraint above and the constraint $C^{\tau}_t(L) \in \big(
(S_{t \wedge \tau}-L)_+,S_{t \wedge \tau}\big)$ are both satisfied.
Again by the convexity constraint, we must have
\[
\frac{S_{t \wedge \tau} - C^{\tau}_t(L)}{0-L} < \frac{C^{\tau}_t(L) - C^{\tau}_t(K)}{L-K} < 0 \quad \Longleftrightarrow \quad 0 < C^{\tau}_t(L) - C^{\tau}_t(K) < \frac{K - L}{L} \cdot \big( 1 - N_{t \wedge \tau}(L) \big) \cdot S_{t \wedge \tau}
\]
then we can set
\[
\begin{split}
& C^{\tau}_t(L) - C^{\tau}_t(K) = N_{t \wedge \tau}(LK) \cdot \frac{K - L}{L} \cdot \big( 1 - N_{t \wedge \tau}(L) \big) \cdot S_{t \wedge \tau} \\
\Longleftrightarrow \quad & C^{\tau}_t(K) = N_{t \wedge \tau}(L) \cdot S_{t \wedge \tau} - N_{t \wedge \tau}(LK) \cdot \big( 1 - N_{t \wedge \tau}(L) \big) \cdot \frac{K - L}{L} \cdot S_{t \wedge \tau}
\end{split}
\]
where $N_t(LK)$ is an independent positive martingale independent of $W$ and of $N(L)$ and unit-bounded. Therefore, we have
\begin{equation}
C^{\tau}_t(K) = \bigg[ N_{t \wedge \tau}(L) - N_{t \wedge \tau}(LK) \cdot \big( 1 - N_{t \wedge \tau}(L) \big) \cdot \frac{K - L}{L} \bigg] \cdot S_{t \wedge \tau}.
\end{equation}
In order to have $C^{\tau}_t(K) \in \big((S_{t \wedge \tau}-K)_+,S_{t \wedge \tau}\big)$, it must be
\[
\begin{split}
	& 0 < N_{t \wedge \tau}(L) - N_{t \wedge \tau}(LK) \cdot \big( 1 - N_{t \wedge \tau}(L) \big) \cdot \frac{K - L}{L} < 1 \\
	\Longleftrightarrow \quad & - \frac{L}{K-L} < 0 < N_{t \wedge \tau}(LK) < \frac{N_{t \wedge \tau}(L)}{1-N_{t \wedge \tau}(L)} \cdot \frac{L}{K-L}.
\end{split}
\]
Therefore, if we
\begin{itemize}
	\item assume $S_0 < L < K$ and $N_0(LK) < \frac{N_0(L)}{1-N_0(L)} \frac{L}{K-L}$ continuous;
	\item redefine $\tau := \inf \Big\{ t \in ]0,T[: S_t = L \, \vee \, N_t(LK) = \frac{N_t(L)}{1-N_t(L)}\cdot \frac{L}{K-L} \Big\}$;
\end{itemize}
then the market is arbitrage-free on $[0,\tau] \, \cup \, \{T\}$.
