# Supplementary material for: Revisiting the Implied Remaining Variance framework of Carr and Sun (2014): Locally consistent dynamics and sandwiched martingales
Source: arXiv:2105.06390 source file (2021-05-13)
Supplement: Supplementary file 2 [file Appendix_old.tex]

\begin{appendices}

%\section{Example of consistent dynamics}
%\label{app:CScondyn}

%	Based on the discussion made in Section~\ref{sec:Carr}, we propose to modify the IRV dynamics of Eq.~\eqref{eq:CSdw} in the following way
%	\begin{equation}\label{eq:appCSdw}
%		\begin{cases}
%			dF_t = \sigma_t F_t \, dW_t \\
%			d\omega_t(K) = - \Big[1 - a_0 + a_1 \, \omega_t(K)\Big] \sigma_t^2 \, dt + \omega_t(K) \, \sigma_t \, dZ_t \\
%			d\langle W, Z\rangle_t = \rho_t \, dt
%		\end{cases}
%	\end{equation}
%	where now $\rho_t$ is a stochastic process defined as
%	\[
%	\rho_t \coloneqq 
%	\begin{cases}
%		-1 & \text{if $k_t > 2$} \\
%		- k_t / 2 & \text{if $k_t \in [-2,2]$} \\
%		+1 & \text{if $k_t < -2$}
%	\end{cases}.
%	\]
	
%	Under the assumptions
%	\begin{gather*}
%		a_0 > 1 \\
%		a_1 \ge 1/4
%	\end{gather*}
%	Eq.~\eqref{eq:CSrightsol} and~\eqref{eq:CSdw2} are still valid, in the form
%	\begin{gather}
%		\omega_t(K) = 2 \Big(2 \rho_t - 1 - 4 a_1 + \sqrt{D_t} \Big) \notag \\
%		\label{eq:appCSdw2} d\omega_t(K) = \frac{1}{\sqrt{D_t}} \, \bigg[ 1 + 2 \rho_t + k_t - \frac{(2 \rho_t + k_t)^2}{D_t} \bigg] \, \sigma_t^2 \, dt - 2 \, \frac{2 \rho_t + k_t}{\sqrt{D_t}} \, \sigma_t \, \bigg( \frac{1}{\rho_t} \, dZ_t - \sqrt{\frac{1}{\rho^2}-1} \, dW_t^{\bot} \bigg)
%	\end{gather}

%	Now, when $k_t > 2$, we have $\rho_t = -1$ and we know from Section~\ref{sec:Carr} that
%	\[
%	\omega_t(K) = - \big(3 + 4 a_1 \big) + \sqrt{\big(3 + 4 a_1 \big)^2 + 4 \big(k_t - 2 \big)}
%	\]
%	is the unique positive solution of the system
%	\[
%	\begin{cases}
%		\omega_t(K) = 2 \Big(2 \rho_t - 1 - 4 a_1 + \sqrt{D_t} \Big) \\
%		\omega_t(K) = 2 \frac{k_t - 2}{\sqrt{D_t}}.
%	\end{cases}
%	\]

\section{Sandwiched martingales with three calls}
\label{app:exsan}

	In this appendix we build three sandwiched martingales consistent with an arbitrage-free market where there exist three European call options with strike prices $L < K < J$ and same maturity, $T$. This case is of particular interest because it is the simplest environment in which all the common no-arbitrage constraints come into play. As in Example~\ref{ex:single}, assume that the uncertainty in the market is described by the filtered probability space $\big(\Omega,\mathcal{F},(\mathcal{F}_t)_{t \ge 0},\mathbb{Q}\big)$ and that the underlying asset price dynamics is given by
	\[
	\begin{cases}
		dS_t = \sigma_t S_t \, dW_t \\
		S_0 > 0
	\end{cases}
	\]
	where $W$ is a standard Brownian motion and the positive process $\sigma_t$ satisfies the Novikov condition. This market is arbitrage-free on $[0,\tau] \cup \{T\}$ if $C^{\tau}(L)$, $C^{\tau}(K)$ and $C^{\tau}(J)$ are sandwiched martingales such that:
	\begin{enumerate}
		\item $(S_{t \wedge \tau} - L)_+ < C^{\tau}_t(L) < S_{t \wedge \tau}$;
		\item $(S_{t \wedge \tau} - K)_+ < C^{\tau}_t(K) < S_{t \wedge \tau}$;
		\item $(S_{t \wedge \tau} - J)_+ < C^{\tau}_t(J) < S_{t \wedge \tau}$;
		\item $C^{\tau}_t(J) < C_t(K) < C^{\tau}_t(L)$;
		\item $-1 < \frac{C^{\tau}_t(L) - C^{\tau}_t(K)}{(L-K)} < \frac{C^{\tau}_t(K)-C^{\tau}_t(J)}{(K-J)} < 0$.
	\end{enumerate}
	Let $A_t$, $B_t$ and $N_t$ be positive martingales bounded by 1 and independent of each other and $W$. We set:
	\begin{align}
		C^{\tau}_t(L) & = (S_{t \wedge \tau}-L)_+ + A_{t \wedge \tau} \cdot \big[S_{t \wedge \tau} - (S_{t \wedge \tau}-L)_+\big] \\
		C^{\tau}_t(K) & = C^{\tau}_t(L) - B_{t \wedge \tau} \cdot (K-L) \\
		C^{\tau}_t(J) & = C^{\tau}_t(K) - N_{t \wedge \tau} \cdot B_{t \wedge \tau} \cdot (J-K).
	\end{align}
	Hence, constraints $1$, $4$ and $5$ are trivially satisfied. About constraints $3$ and $4$, we have
	\[
	\begin{split}
		& (S_{t \wedge \tau} - K)_+ < C^{\tau}_t(K) < S_{t \wedge \tau} \\
		\Longleftrightarrow \quad & \frac{(S_{t \wedge \tau}-K)_+}{A_{t \wedge \tau}} - \bigg(\frac{1}{A_{t \wedge \tau}} - 1\bigg) \cdot (S_{t \wedge \tau}-L)_+ + \frac{B_{t \wedge \tau}}{A_{t \wedge \tau}} \cdot (K-L) < S_{t \wedge \tau} \\
		& < \frac{S_{t \wedge \tau}}{A_{t \wedge \tau}} - \bigg(\frac{1}{A_{t \wedge \tau}} - 1 \bigg) \cdot (S_{t \wedge \tau} -L)_+ + \frac{B_{t \wedge \tau}}{A_{t \wedge \tau}} \cdot (K-L)
	\end{split}
	\]
	and
	\[
	\begin{split}
		& (S_{t \wedge \tau} - J)_+ < C^{\tau}_t(J) < S_{t \wedge \tau} \\
		\Longleftrightarrow \quad & \frac{(S_{t \wedge \tau}-J)_+}{A_{t \wedge \tau}} - \bigg(\frac{1}{A_{t \wedge \tau}} - 1\bigg) \cdot (S_{t \wedge \tau}-L)_+ + \frac{B_{t \wedge \tau}}{A_{t \wedge \tau}} \cdot (K-L) + \frac{N_{t \wedge \tau} \cdot B_{t \wedge \tau}}{A_{t \wedge \tau}} \cdot (J-K) < S_{t \wedge \tau} \\
		& < \frac{S_{t \wedge \tau}}{A_{t \wedge \tau}} - \bigg(\frac{1}{A_{t \wedge \tau}} - 1 \bigg) \cdot (S_{t \wedge \tau} -L)_+ + \frac{B_{t \wedge \tau}}{A_{t \wedge \tau}} \cdot (K-L) + \frac{N_{t \wedge \tau} \cdot B_{t \wedge \tau}}{A_{t \wedge \tau}} \cdot (J-K).
	\end{split}
	\]
	Therefore, if we define the stopping time $\tau$ as
	\[
	\begin{split}
	\tau \coloneqq \inf \bigg\{ t \in (0,T): & \, S_t \le \mathcal{M} - \bigg(\frac{1}{A_{t \wedge \tau}} - 1\bigg) \cdot (S_{t \wedge \tau}-L)_+ + \frac{B_{t \wedge \tau}}{A_{t \wedge \tau}} \cdot (K-L) \\
	\vee \, & S_t \ge \frac{S_{t \wedge \tau}}{A_{t \wedge \tau}} - \bigg(\frac{1}{A_{t \wedge \tau}} - 1 \bigg) \cdot (S_{t \wedge \tau} -L)_+ + \frac{B_{t \wedge \tau}}{A_{t \wedge \tau}} \cdot (K-L) \bigg\},
	\end{split}
	\]
	where $\mathcal{M} = \max\Big\{\frac{(S_{t \wedge \tau}-K)_+}{A_{t \wedge \tau}}, \frac{(S_{t \wedge \tau}-J)_+}{A_{t \wedge \tau}}+ \frac{N_{t \wedge \tau} \cdot B_{t \wedge \tau}}{A_{t \wedge \tau}} \cdot (J-K)\Big\}$, and we assume that $S_0$ is in the proper region, then we have that the market is arbitrage-free on $[0,\tau] \cup \{T\}$.
	
\end{appendices}
